# Supplementary material for: FoldToken: Learning Protein Language via Vector Quantization and Beyond
Source: arXiv:2403.09673 source file (2024-03-19)
Supplement: Supplementary file 1 [file FoldToken_appendix.pdf]

## A. Folding Angle Definition

As shown in Fig. 5, following the backbone direction, given the previous three atoms, we can construct a local frame  $T_u = \{\mathbf{x}_i, \mathbf{x}_j, \mathbf{x}_k\}$ . The next atom  $\mathbf{x}_u$  can be represented by the distance  $r_u$  and two torsion angles  $\alpha_u$  and  $\beta_u$ , denoted as  $\mathbf{a}_u = (r_u, \alpha_u, \beta_u)$ .

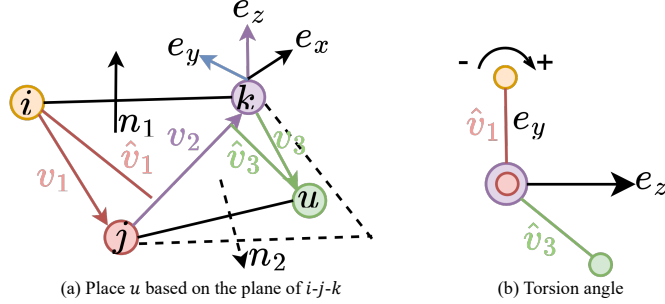

Figure 5: Torsion angle computation.

**Structure as angle sequence** The vanilla protein structures are represented as 3d points, where the rotation and translation equivariance should be considered in modeling. To directly apply the transformer-based encoder and decoder, we convert the 3d points into a sequence of angles, which is rotation and translation invariant. As shown in Fig. 5, following the backbone direction, given previous three atoms, we can construct a local frame  $T_u = \{\mathbf{x}_i, \mathbf{x}_j, \mathbf{x}_k\}$ . The next atom  $\mathbf{x}_u$  can be represented by the distance  $r_u$  and two torsion angles  $\alpha_u$  and  $\beta_u$ , denoted as  $\mathbf{a}_u = (r_u, \alpha_u, \beta_u)$ .

$$\begin{cases} \mathbf{v}_1 = \mathbf{x}_j - \mathbf{x}_i \\ \mathbf{v}_2 = \mathbf{x}_k - \mathbf{x}_j \\ \mathbf{v}_3 = \mathbf{x}_u - \mathbf{x}_k \\ \hat{\mathbf{v}}_1 = -\mathbf{v}_1 - ((-\mathbf{v}_1) \cdot \mathbf{v}_2)\mathbf{v}_2 \\ \hat{\mathbf{v}}_3 = \mathbf{v}_3 - (\mathbf{v}_3 \cdot \mathbf{v}_2)\mathbf{v}_2 \\ r_u = \|\mathbf{v}_3\|_2 \\ \alpha_u = \angle(-\hat{\mathbf{v}}_2, \hat{\mathbf{v}}_3) \\ \beta_u = \angle(\hat{\mathbf{v}}_1, \hat{\mathbf{v}}_3) = \angle(\mathbf{n}_1, \mathbf{n}_2) \end{cases} \quad (16)$$

To completely represent the structure, we add virtual frames  $T_0$  and  $T_{n+1}$  at the start and end of the protein structure, where the virtual atoms have fixed  $(r, \alpha, \beta) = (1, 1, 1)$  to its nearest backbone frames. Finally, the protein structure  $\mathcal{X} = \{\mathbf{x}_i \in \mathbb{R}^3 : 1 \leq i \leq n\}$  will be represented as  $\mathcal{S} = \{(r_i, \alpha_i, \beta_i) : 0 \leq i \leq n+1\}$ .

## B. Local Metrics for Backbone Inpainting

We define the average recovering loss per residue:

$$\begin{cases} L_r = \frac{1}{b} \sum_{i=1}^b \sum_{j=1}^{n_i} \frac{|r_{i,j} - \hat{r}_{i,j}|}{n_i} \\ L_\alpha = \frac{1}{b} \sum_{i=1}^b \sum_{j=1}^{n_i} \frac{|\alpha_{i,j} - \hat{\alpha}_{i,j}|}{n_i} \\ L_\beta = \frac{1}{b} \sum_{i=1}^b \sum_{j=1}^{n_i} \frac{|\beta_{i,j} - \hat{\beta}_{i,j}|}{n_i} \end{cases} \quad (17)$$

where  $b$  is batch size and  $n_i$  is the length of protein  $i$ . The maximum recovering loss per residue is:

$$\begin{cases} \max L_r = \frac{1}{b} \sum_{i=1}^b \max_{j=1}^{n_i} |r_{i,j} - \hat{r}_{i,j}| \\ \max L_\alpha = \frac{1}{b} \sum_{i=1}^b \max_{j=1}^{n_i} |\alpha_{i,j} - \hat{\alpha}_{i,j}| \\ \max L_\beta = \frac{1}{b} \sum_{i=1}^b \max_{j=1}^{n_i} |\beta_{i,j} - \hat{\beta}_{i,j}| \end{cases} \quad (18)$$

## C. Reconstruction Visualization

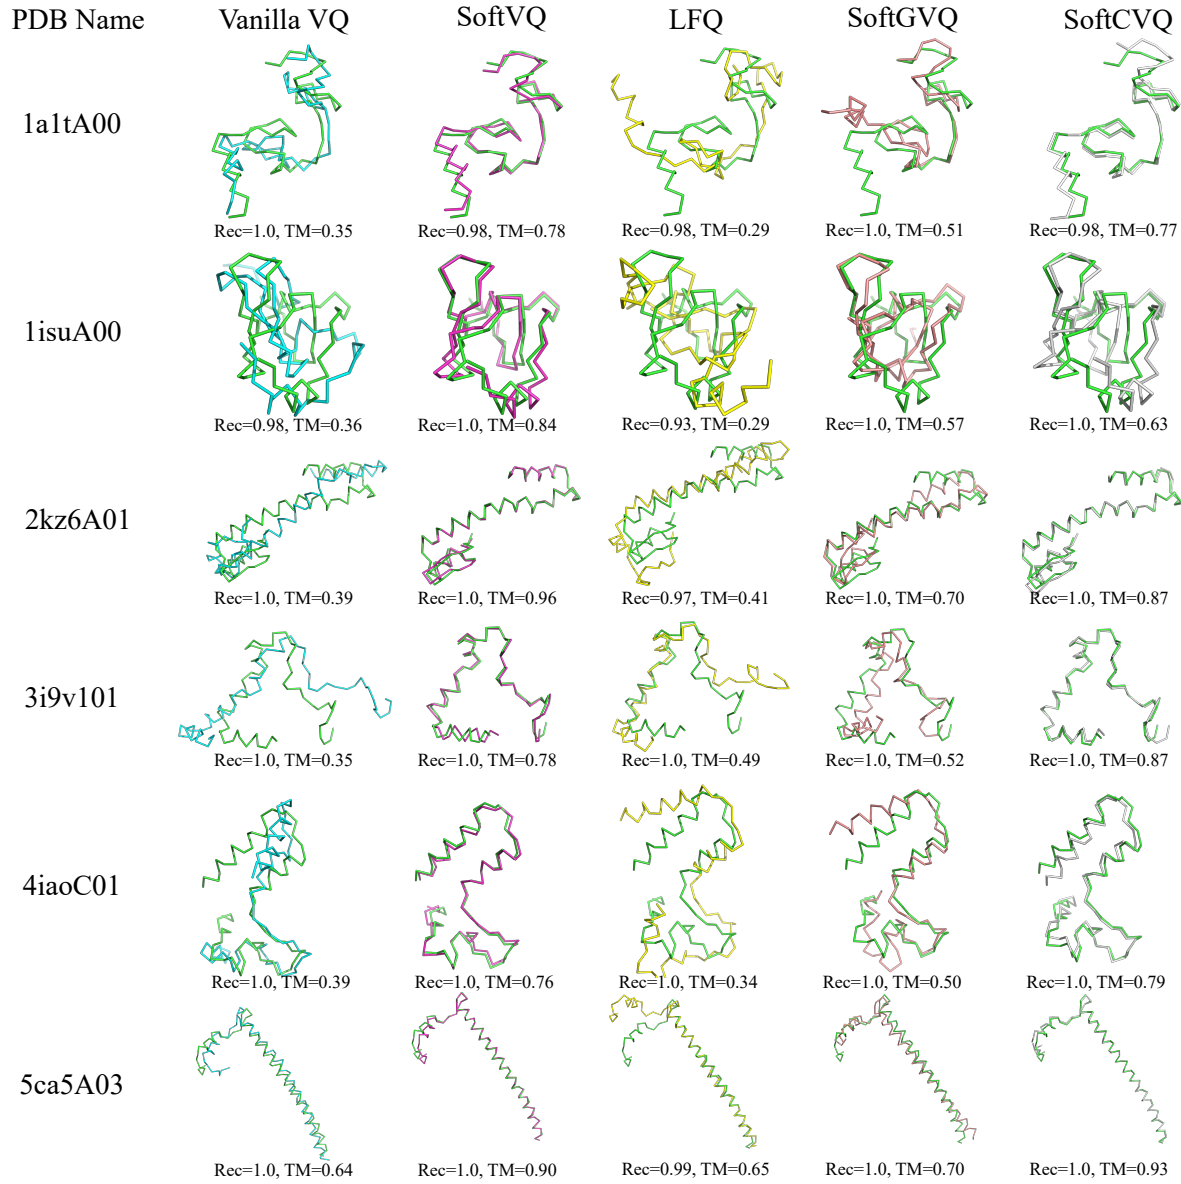

**Figure 6:** Reconstructed examples.

## D. Ablation of SoftCVQ

We investigate the impact of the number of MLP layers (#MLP), the dimension of the codebook vector (#CodeDim), and spherical normalization (sphere) on the reconstruction performance of SoftCVQ. Table 5 demonstrates that appropriately increasing #MLP and #CodeDim enhances performance. Additionally, we highlight the significance of spherical normalization in achieving optimal results.

| Method-ID | Config |          | Sphere | Global Metrics |         | Success Rates   |                    |
|-----------|--------|----------|--------|----------------|---------|-----------------|--------------------|
|           | #MLP   | #CodeDim |        | Rec            | TMScore | Rec $\geq$ 0.95 | TMScore $\geq$ 0.5 |
| SCQ-1     | 2      | 16       |        | 0.9801         | 0.5853  | 0.8997          | 0.7638             |
| SCQ-2     | 2      | 16       | ✓      | 0.9879         | 0.6451  | 0.9572          | 0.8892             |
| SCQ-3     | 2      | 32       |        | 0.9965         | 0.4285  | 0.9937          | 0.2184             |
| SCQ-4     | 2      | 32       | ✓      | 0.9896         | 0.6959  | 0.9561          | 0.9216             |
| SCQ-5     | 3      | 32       |        | 0.9875         | 0.5867  | 0.9457          | 0.7367             |
| SCQ-6     | 3      | 32       | ✓      | 0.9862         | 0.6697  | 0.9467          | 0.9028             |
| SCQ-7     | 6      | 32       | ✓      | 0.9880         | 0.7470  | 0.9603          | 0.9498             |
| SCQ-8     | 9      | 32       | ✓      | 0.9875         | 0.7015  | 0.9551          | 0.9101             |

**Table 5:** Ablation of SoftCVQ on CATH4.3 test set.
